# Supplementary material for: Layering instability in a confined suspension flow
Source: arXiv:1111.4538 source file (2011-11-19)
Supplement: Supplementary file 1 [file supplemental_document.pdf]

# Supplemental Materials for "Layering instability in a confined suspension flow"

This Supplemental Document is organized into three sections. Movies that show results of our direct numerical simulations of confined suspensions at different particle concentrations are described in Sec. 1. Further details on our methods that have been used to analyze particle dynamics in dilute suspensions in Couette flow are provided in Secs. 2 and 3: Sec. 2 presents our Boltzmann–Monte Carlo (BMC) simulation technique, and Sec. 3 describes our simplified three-dimensional collision model M3.

## 1. Movies – Suspension dynamics at different concentrations

In this section we describe movies that show results of our direct numerical simulations of suspensions in Couette flow between two planar walls at low and moderate concentrations. The movies support our theoretical analysis presented in the Letter. Movies **A 1**–**A 4** illustrate the layering phenomenon predicted by our theoretical analysis, and Movies **B 1**–**B 4** provide evidence of the role of the swapping trajectory (ST) effect at nonzero particle concentrations.

The simulations were performed using our accelerated Cartesian-representation algorithm [1–3], with multiparticle hydrodynamic interactions (HI) under creeping-flow conditions accurately taken into account. To achieve high accuracy, the algorithm combines the HYDROMULTIPOLE method [4] with an expansion of the flow field interacting with the walls into lateral Fourier modes [1, 2]. The accelerated version of the algorithm also utilizes simplifications associated with the Hele–Shaw asymptotic behavior of the far-field flow in the parallel-plate geometry [5].

In addition to the flow-mediated hydrodynamic interactions, the particles interact via a short-range repulsive potential that mimics direct contacts between rough particles. In all simulations presented in the Supplemental Materials the range of the repulsive potential is $\epsilon = 0.1d$, where $d$ is the particle diameter.

It is assumed that the suspension undergoes a planar Couette flow in the $x$ direction,

$$\mathbf{v} = \dot{\gamma} z \hat{\mathbf{e}}_x, \tag{S1}$$

where $\dot{\gamma}$ is the shear rate, and $\hat{\mathbf{e}}_x$ is the unit vector along the axis $x$. The direction of flow gradient $z$ is normal to the walls, which are at $z = 0$ and $z = H$. No-slip boundary conditions on the wall surfaces are assumed. Our simulations were performed in a periodic box, with periodicity in the lateral directions $x$ and $y$ implemented using the method described in [3].

### A. *Microstructural evolution*

Movies **A 1**–**A 4** present the microstructural evolution at four suspension volume fractions, ranging from $\phi = 0.033$ to $\phi = 0.3$. The videos show the projection of the positions of all particles in a periodic box onto the $y$–$z$ plane (normal to the flow direction). In all cases the suspension develops a layered structure, in agreement with predictions of our theory. At low concentrations, $\phi \lesssim 0.1$ the timescale for the microstructural evolution $\tau_\mathrm{L}$ scales with the inverse of the suspension volume fraction, $\tau_\mathrm{L} \sim \phi^{-1}$, consistent with the binary-collision analysis. At higher concentrations the microstructural evolution occurs on a faster scale.

The movies also indicate that at significantly longer times $t \gg \tau_\mathrm{L}$ another instability occurs, leading to the decomposition of particle layers into string-like structures with a hexagonal order in the $y$–$z$ plane. This instability is not captured by our theory because of the assumed translational invariance in the $y$ direction.

The long-time microstructure observed in our simulations is similar to the one reported at high-volume fractions for unconfined suspensions [6, 7]. We note, however, that in unconfined systems suspension instability occurs only at volume fractions $\phi \gtrsim 0.5$, whereas in confined suspensions, layering occurs at arbitrary concentrations.

*Movie captions* – Movies **A 1**–**A 4** show the evolving suspension microstructure in the vorticity–gradient plane $y$–$z$. The points indicate projections of the particle centers onto this plane. The wall separation is $H/d = 4.4$.

**Movie A 1:** Evolution for $\phi = 0.033$. The layered microstructure is well developed at time $\dot\gamma t \approx 1000$. The total simulation time is $\dot\gamma t_\mathrm{F} = 1200$. Simulation of a system with $N = 900$ particles.

**Movie A 2:** Evolution for $\phi = 0.1$. The layered microstructure is well developed at time $\dot\gamma t \approx 330$. The total simulation time is $\dot\gamma t_\mathrm{F} = 2600$. Simulation of a system with $N = 300$ particles.

**Movie A 3:** Evolution for $\phi = 0.2$. The layered microstructure is well developed at time $\dot\gamma t \approx 120$. The total simulation time is $\dot\gamma t_\mathrm{F} = 550$. Simulation of a system with $N = 300$ particles.

**Movie A 4:** Evolution for $\phi = 0.3$. The layered microstructure is well developed at time $\dot\gamma t \approx 30$. The total simulation time is $\dot\gamma t_\mathrm{F} = 670$. Simulation of a system with $N = 300$ particles.

### B. *Swapping trajectory effect*

Movies **B 1**–**B 4** illustrate the ST effect in a confined suspension at volume fractions ranging from $\phi = 0.003$ to $\phi = 0.2$. The videos show the projection of particle contours onto the $x$–$z$ plane in the coordinate system relative to one of the particles in a randomly chosen

pair (shown in blue). All other particles with centers within a prescribed box around the selected central particle are shown in red.

The blue particle pair is chosen based on the condition that the selected particles are within a swapping distance at the initial time. Each movie shows a sequence of several encounters of randomly selected pairs of particles. The random selection allows us to illustrate typical particle behavior, without introducing a significant subjective bias. The key parameters of our simulations are given in the captions below, and further details are available from the authors upon request.

The sequence of trajectories shown in Movie **B 1** demonstrates that at low particle concentrations (below volume fraction $\phi = 0.01$), particles perform well-defined swapping motions, i.e., the particles initially approach each other, but then change streamlines and separate without a collision. The trajectory sequences shown in movies **B 2**–**B 4** indicate that as the suspension concentration increases the trajectories fluctuate with growing intensity, as a result of the interactions of a given particle pair with the surrounding particles. However, the essential features of the ST mechanism remain present in all cases studied: due to the wall-induced hydrodynamic lift, particles migrate from the collisional to non-collisional streamlines, leading, on average, to the reversal of particle motion, and a significant reduction of collision frequency.

*Movie captions* – Movies **B 1**–**B 4** show relative trajectories for pairs of particles (shown in blue) with configurations within the swapping range.

**Movie B 1:** Sequence of trajectories for $\phi = 0.003$. The initial relative position of the blue particles is within the domain $5 < \Delta x_{\rm b}/d < 6$, $0 < \Delta y_{\rm b}/d < 0.1$, and $0.15 < \Delta z_{\rm b}/d < 0.2$. Other particles within the box $\Delta x_{\rm r}/d < 6$, $\Delta y_{\rm r}/d < 0.8$, and $\Delta z_{\rm r}/d < 3$ are shown in red. Wall separation $H/d = 5$.

**Movie B 2:** Sequence of trajectories for $\phi = 0.025$. The initial position of blue particles is in the domain $3.5 < \Delta x_{\rm b}/d < 4$, $0 < \Delta y_{\rm b}/d < 0.1$, and $0.15 < \Delta z_{\rm b}/d < 0.2$. Other particles within the box $\Delta x_{\rm r}/d < 4$, $\Delta y_{\rm r}/d < 0.8$, and $\Delta z_{\rm r}/d < 3$ are shown in red. Wall separation $H/d = 5$.

**Movie B 3:** Sequence of trajectories for $\phi = 0.1$. The initial position of blue particles is in the domain $1.5 < \Delta x_{\rm b}/d < 2$, $0 < \Delta y_{\rm b}/d < 0.1$, and $0.1 < \Delta z_{\rm b}/d < 0.15$. Other particles within the box $\Delta x_{\rm r}/d < 3$, $\Delta y_{\rm r}/d < 0.8$, and $\Delta z_{\rm r}/d < 3$ are shown in red. Wall separation $H/d = 5$.

**Movie B 4:** Sequence of trajectories for $\phi = 0.2$. The initial position of blue particles is in the domain $1.5 < \Delta x_{\rm b}/d < 2$, $0 < \Delta y_{\rm b}/d < 0.1$, and $0.15 < \Delta z_{\rm b}/d < 0.2$. Other particles within the box $\Delta x_{\rm r}/d < 3$, $\Delta y_{\rm r}/d < 0.8$, and $\Delta z_{\rm r}/d < 3$ are shown in red. Wall separation $H/d = 4.4$.

## 2. Boltzmann Monte Carlo method for dilute suspensions

The BMC method is a general computer simulation technique that describes the evolution of a dilute particulate system in terms of a sequence of uncorrelated binary collisions (similar to the evolution of a Boltzmann gas). In this method, particle distribution is represented by an ensemble of $N$ independent particles. The ensemble is updated in time by performing binary collisions of randomly chosen particles.

In our present study this method is used to simulate the evolution of the particle distribution in a dilute suspension undergoing planar Couette flow (S1) between two parallel walls normal to the $z$ direction. In our implementation of the BMC method it is assumed that the suspension is uniform in the flow and vorticity directions $x$ and $y$. Under these conditions the system can be described by the one-particle density $n(z,t)$ that depends only on the transverse position $z$ and time $t$. The distribution $n(z,t)$ is represented by an ensemble of $N$ independent particles, each with an assigned value of the coordinate $z$ (but with no assigned values of the coordinates $x$ and $y$).

Initially, the positions $z_i$ of particles $i = 1, \ldots, N$ are assigned randomly, with a uniform probability distribution in the space between the walls. The evolution of the particle ensemble is then generated by carrying out a sequence of binary collisions with a large initial offset in the streamwise direction, $\Delta x_{ij} = x_i - x_j \gg d$ (where $d$ is the particle diameter), and an offset in the vorticity direction, $\Delta y_{ij} = y_i - y_j$, assigned randomly. In our calculations, each collision event consists of the following operations:

- A pair of particles $i, j$ is randomly chosen, with a probability proportional to their relative velocity at infinite streamwise separation $\Delta x_{ij}$ and given positions $z_i$ and $z_j$. This non-uniform probability distribution accounts for the dependence of the frequency of particle collisions on the velocity of the mutual approach.
- Particle offset in the vorticity direction $\Delta y_{ij}$ is chosen randomly with a uniform distribution.
- The post-collision particle positions are evaluated from the pre-collision offsets $\Delta y_{ij}$ and positions $z_i$ and $z_j$, by either (a) simulating the exact two-particle trajectory (BMC-HI) or (b) using a simplified collision model M2 or M3.
- The transverse coordinates $z_i$ and $z_j$ of the particles involved in the collision event are updated according to their post-collision values.

We use the BMC method in two ways: (a) to describe suspension evolution for a system with the exact pair dynamics of hydrodynamically interacting particles (BMC-HI), and (b) to solve the population-balance equations for two simplified binary-collision models, M2 and M3. The HI are accurately evaluated using methods explained in Sec. 1. The simplified models: M2 [defined in Eq. (2) in the Letter] and M3 [defined in Eq. (S4)] are constructed

to preserve the essential features of binary collisions (especially, the effect of swapping trajectories), without incurring high numerical cost of the full hydrodynamic calculations.

### 3. Collision model M3

Model M3 generalizes the two-dimensional (2D) collision model M2 to three dimensions. M3 is governed by equations that are analogous to the 2D population-balance equation (1) and the binary-collision kernel (2). The three-dimensional version of the population-balance equation (1) is

$$\frac{\partial n(z,t)}{\partial t} = \dot{\gamma}\int_{-\infty}^{\infty} [n(z+\tfrac{1}{2}\Delta z-\tfrac{1}{2}\Delta z')n(z-\tfrac{1}{2}\Delta z-\tfrac{1}{2}\Delta z') - n(z)n(z-\Delta z)]\,\Delta z\, d\Delta y\, d\Delta z, \tag{S2}$$

where $\Delta y$ and $\Delta z$ are the pre-collision particle offsets in the vorticity and gradient directions, and

$$\Delta z' = \Delta z'(\Delta y, \Delta z) \tag{S3}$$

is the post-collision offset in the gradient direction. As in our BMC calculations described in Sec. 2, we assume in Eq. (S2) that the particle density $n(z,t)$ is independent of the coordinates $x$ and $y$. It is also assumed that the displacements of the two colliding particles are symmetric.

As with usual population-balance equations [8], the first term on the right-hand side of Eq. (S2) is the gain term. It corresponds to a particle with the initial position $z_1 = z+\frac{1}{2}\Delta z-\frac{1}{2}\Delta z'$ arriving at the position $z_1' = z$ after a collision with another particle initially at $z_2 = z-\frac{1}{2}\Delta z-\frac{1}{2}\Delta z'$. The second term is the loss term, corresponding to a particle removed from the position $z$ after a collision.

The simplified model M3 for the collision kernel (S3) neglects the hydrodynamic interactions for particles on the collision trajectories, but preserves a finite swapping region that prevents direct contacts of particles that have sufficiently small offsets $\Delta y$ and $\Delta z$. Specifically, in model M3 the post-collision offset $\Delta z'$ in the gradient direction is

$$\Delta z' = \begin{cases} -\Delta z, & 0<|\Delta z|<\kappa_s, \\ \dfrac{\kappa_c \Delta z}{(\Delta y^2+\Delta z^2)^{1/2}}, & \kappa_s<|\Delta z|, \quad \Delta y^2+\Delta z^2<\kappa_c^2, \\ \Delta z, & \kappa_c^2<\Delta y^2+\Delta z^2<\infty. \end{cases} \tag{S4}$$

Following the results of our detailed hydrodynamic analysis presented in [9], the swapping range $\kappa_s$ in relation (S4) is independent of the initial particle separation in the vorticity direction, $\Delta y$. The post-collision displacement of particles on collisional trajectories [the middle case in (S4)] stems from the assumption that the particles follow streamlines of the unperturbed external flow until arriving at the contact position, and subsequently they slide

over each other under the action of the central repulsive force. During this process the projection $(\Delta y, \Delta z)$ of the relative particle position is moving in the radial direction, until the separation distance $\Delta y^2 + \Delta z^2 = \kappa_c^2$ is achieved.

---

[1] S. Bhattacharya, J. Bławzdziewicz, and E. Wajnryb, Physica A **356**, 294 (2005).

[2] M. Baron, J. Bławzdziewicz, and E. Wajnryb, Phys. Rev. Lett. **100**, 174502 (2008).

[3] J. Bławzdziewicz and E. Wajnryb, Phys. Fluids. **20**, 093303 (2008).

[4] B. Cichocki, B. U. Felderhof, K. Hinsen, E. Wajnryb, and J. Bławzdziewicz, J. Chem. Phys. **100**, 3780 (1994).

[5] S. Bhattacharya, J. Bławzdziewicz, and E. Wajnryb, J. Comput. Phys. **212**, 718 (2006).

[6] A. Sierou and J. Brady, J. Rheol. **46**, 1031 (2002).

[7] S. Kulkarni and J. Morris, J. Rheol. **53**, 417 (2009).

[8] D. Ramkrishna, *Population Balances: Theory and Applications to Particulate Systems in Engineering* (Academic Press, San Diego, California, 2000).

[9] M. Zurita-Gotor, J. Bławzdziewicz, and E. Wajnryb, J. Fluid Mech. **592**, 447 (2007).
